# Supplementary material for: Detection Transformer with Stable Matching
Source: arXiv:2304.04742 source file (2023-04-10)
Supplement: Supplementary file 1 [file appendix_experiments.tex]

\begin{table*}[ht]
\centering\setlength{\tabcolsep}{7pt}

\footnotesize
\vspace{-3mm}
{
\resizebox{0.8\textwidth}{!}{%
\begin{tabular}{l|l|c|cccccc}
\shline
Model & Backbone & \#epochs  & AP & AP$_{50}$ & AP$_{75}$ & AP$_{S}$ & AP$_{M}$ & AP$_{L}$\\
\shline
Deformable-DETR~\cite{zhu2020deformable} & R50 & $12$ & $56.1$ & $75.2$ & $61.3$ & $39.3$ & $60.4$ & $72.4$ \\
\rowcolor{gray!15} Stable-Deformable-DETR (ours) & R50  & $12$ & ${57.6}$ & ${76.5}$ & ${63.2}$ & ${41.4}$ & ${61.7}$ & ${73.9}$\\
\shline
DAB-Deformable-DETR~\cite{liu2022dabdetr} & R50  & $12$ & ${56.9}$ & ${75.5}$ & ${62.6}$ & ${40.1}$ & ${61.2}$ & ${73.3}$\\
\rowcolor{gray!15} Stable-DAB-Deformable-DETR (ours) & R50 & $12$ & $56.8$ & $75.6$ & $62.0$ & $40.0$ & $60.5$ & $73.2$ \\
\shline
$\mathcal{H}$-DETR~\cite{HDETR} & R50 & $12$ & $48.6$ & ${66.8}$ & ${52.9}$ & $30.7$ & $51.8$ & $63.5$ \\
\rowcolor{gray!15} Stable-$\mathcal{H}$-DETR (ours) & R50 & $12$ & $58.0$ & ${77.1}$ & ${66.3}$ & $41.3$ & $62.1$ & $73.6$ \\
\shline
\end{tabular}}
\vspace{-0.2cm}
\caption{{The full results of the effectiveness of our methods on DETR variants. The models with prefix "Stable" use our proposed methods.}}
\label{tab:effectiveness_full_results}
}
\end{table*}
